# Supplementary material for: The Network Propensity Score: Spillovers, Homophily, and Selection into Treatment
Source: arXiv:2209.14391 source file (2022-09-28)
Supplement: Supplementary file 1 [file proofsappendix.tex]

\subsection{Proofs Appendix}

\begin{proof}[Proof of Lemma \ref{lem:momentsdbar} (\nameref{lem:momentsdbar}):]
	In order to have a well-defined expectation, I condition only on realizations of $G_{ig}$ for which $L_{ig} \equiv \sum_{jg} G_{ijg} > 0$. Furthermore, let $Z_{ig} \equiv (W_{ig},A_{ig},\Psi_g)$ and $z \equiv (w,a,\Psi)$ denote a specific realization. Therefore we can write the conditional expectation as
	\begin{align*}
	\mathbb{E}[\bar{D}_{-ig} \mid G_{ig},z] &= \mathbb{E}\left[\left( \sum_{j \ne i} G_{ijg}D_{ijg}\right)/L_{ig} \mid G_{ig}, z\right] &\text{(Definition $\bar{D}_{ig}$)} \\
	&= \left(\sum_{j \ne i} G_{ijg}\mathbb{E}\left[D_{ijg} \mid G_{ijg}=1,G_{ig}, z\right]\right)/L_{ig} &\text{(Distribute Expectation)} \\
	&= \left(\sum_{j \ne i} G_{ijg}\mathbb{E}\left[D_{ijg} \mid G_{ijg} = 1, z\right]\right)/ L_{ig} &\text{(Equation \ref{eq:proofjointprob})} \\
	&= p_f(z) &\text{(Grouping Terms)}
	\end{align*}
	We can use similar ideas to compute the second moment. For two distinct individuals $j \ne j'$, \eqref{eq:proofjointprob} implies that $\mathbb{E}[D_{jg}D_{j'g} \mid G_{ig},z] = p_f(z)p_f(z)$.		
	\begin{align*}
	&\mathbb{E}[\bar{D}_{-ig}^2 \mid G_{ig},z] \\
	&= \mathbb{E}\left[\left(\sum_{j,j' \ne i}G_{ijg}G_{ij'g}D_{jg}D_{j'g}\right)/L_{ig}^2 \mid G_{ig},z\right] &\text{(Definition $\bar{D}_{ig}^2$)} \\
	&= \left(\sum_{j,j' \ne i}G_{ijg}G_{ij'g}\mathbb{E}\left[D_{jg}D_{j'g} \mid G_{ig},z\right]\right)/L_{ig}^2 &\text{(Distribute Expectations)} \\
	&= \left(\sum_{j,j' \ne i}G_{ijg}G_{ij'g}\left(\mathbbm{1}\{j = j'\}p_f(z) + \mathbbm{1}\{j \ne j'\}p_f(z)^2\right)\right)/L_{ig}^2 &\text{(Equation \ref{eq:proofjointprob})} \\
	&= \frac{p_f(z)(1-p_f(z))}{L_{ig}^2} + p_f(z)^2  &\text{(Canceling terms)}
	\end{align*}
	
\end{proof}

\begin{proof}[Proof of Corollary \ref{cor:coarsestbalancing} (Coarsest Balancing Score)]
	Define $Z \equiv (W,A,\Psi)$. For simplicity I will denote the conditional CDF, $F_{\{X_{ig} \mid Z_{ig}\}}(x \mid z)$, as $F(x \mid z)$. Suppose that $b(\cdot)$ is a balancing score. Then for a pair of realizations $\{z,z^*\}$ in the support,
	\begin{equation}
	b(z) = b(z^*) \implies	F(x \mid b(z)) = F(x \mid z) = F(x \mid z^*).
	\label{eq:defnbalancing}
	\end{equation}
	Furthermore, if $p(\cdot)$ is the coarsest balancing score, then for all balancing scores $b(\cdot)$, 
	\begin{equation}
	b(z) = b(z^*) \implies p(z) = p(z^*).
	\label{eq:defncoarsest}
	\end{equation}
	
	\begin{enumerate}[(i)]
		\item If $X_{ig} = D_{ig}$, then $\{p_d\}$ is the coarsest score.
		
		Since $X_{ig}$ is binary, the conditional CDF is a Bernoulli distribution with parameter $p_d(w,a)$. Therefore, $p_d(z)$ is a balancing score. Now suppose that $b(z) = b(z^*)$ for an arbitrary balancing score $b(\cdot)$. Equation  \eqref{eq:defnbalancing} implies that $F(x \mid z ) = F(x \mid z^*)$. Since the conditional distribution is completely determined by the propensity score, then $p_d(z) = p_d(z^*)$. Therefore, $\{p_d\}$ satisfies the definition of the coarsest balancing score in \eqref{eq:defncoarsest}. The proof follows the same argument as in \citet{rosenbaum1983central}.		
		
		\item If $X_{ig} = \bar{D}_{-ig}$, then $\{p_\ell,p_{f}\}$ is the coarsest score.
		
		I start by deriving the conditional moments of $\bar{D}_{-ig}$ given $z$. I restrict attention to cases with $p_\ell(z),p_f(z) \in (0,1]$ because otherwise the distribution of $\bar{D}_{-ig}$ is degenerate at $\{0\}$.
		
		By the law of iterated expectations $\mathbb{E}[\bar{D}_{ig} \mid z] = \mathbb{E}[\mathbb{E}[\bar{D}_{ig} \mid G_{ig},z]\mid z]$. We can compute the inner expectation using the first part of Lemma \ref{lem:momentsdbar}. Since we define $\bar{D}_{ig} = 0$ for isolated individuals, then
		
		\begin{equation}
		\label{eq:k1coarsest}
		K_1 \equiv \mathbb{E}[\bar{D}_{ig} \mid z] = (1-(1-p_{\ell}(z))^n)p_f(z).
		\end{equation}
		
		Let $L_{ig}$ denote the total number of links. By the law of iterated expectations and the second part of Lemma \ref{lem:momentsdbar}
		\begin{align*}
			\mathbb{E}[\bar{D}_{-ig}^2\mid z] &= (1-(1-p_{\ell}(z))^n) \times \\
			&\left( \mathbb{E}\left[L_{ig}^{-1} \mid L_{ig} > 0, z \right]p_f(z)(1-p_f(z))+ p_f(z)^2\right)
		\end{align*}
		Therefore, the ratio of the second to the first conditional moments is equal to
		\begin{equation}
		K_2 \equiv \frac{\mathbb{E}[\bar{D}_{-ig}^2\mid z]}{\mathbb{E}[\bar{D}_{-ig}\mid z]} = \mathbb{E}\left[L_{ig}^{-1} \mid L_{ig} > 0, z \right](1-p_f(z))+ p_f(z)
		\label{eq:ratiobalancingscore}
		\end{equation}
		Rearranging equation \eqref{eq:k1coarsest}, $p_f(z) = K_1 / (1-(1-p_\ell(z))^n)$, which means that
		\begin{equation}
		K_2 = \underbrace{\mathbb{E}\left[L_{ig}^{-1} \mid L_{ig} > 0,z\right]}_{(A)}\underbrace{\left(1-\frac{K_1}{1-(1-p_\ell(z))^n}\right)}_{(B)}+\underbrace{\frac{K_1}{1-(1-p_\ell(z))^n}}_{(C)}.
		\label{eq:coarsestk2}
		\end{equation}
		The quantity $(A)$ is contained in $(1/n,1]$. The upper bound is achieved when $\{ig\}$ has one friend, whereas the lower bound, $(1/n)$ is achieved when $\{ig\}$ has $n$ friends. Since $p_f(z') \in (0,1]$ then \eqref{eq:ratiobalancingscore} implies that $(B)$ and $(C)$ are non-negative, and strictly positive for interior values.

		I will show that the right hand-side of \eqref{eq:coarsestk2} is strictly decreasing in $p_{\ell}(z)$. This shows that for a given $(K_1,K_2)$ there exists a unique $p_{\ell}(z)$ that solves \eqref{eq:coarsestk2}. Differentiating,
		\[
		\frac{\partial A}{\partial p_\ell}B + A\frac{\partial B}{\partial p_\ell} + \frac{\partial C}{\partial p_\ell}
		\]
		The derivative $\frac{\partial A}{\partial p_\ell}$ is strictly negative because increasing the link formation probability (first-order stochastically) shifts the degree distribution ($L_{ig}$) to the right. Furthermore, $\frac{\partial B}{\partial p_\ell} = -\frac{\partial C}{\partial p_\ell}$ by construction and $\frac{\partial C}{\partial p_\ell} < 0$. Consequently, $A\frac{\partial B}{\partial p_\ell} + \frac{\partial C}{\partial p_\ell} = (1-A) \frac{\partial C}{\partial p_\ell} < 0$ and the overall derivative is strictly negative.
		
		Suppose that $b$ is an arbitrary balancing score and that $b(z) = b(z')$. Let $(K_1',K_2')$ denote the conditional moments given $z'$.
		
		Since $b$ is a balancing score, then $(K_1,K_2) = (K_1',K_2')$ because their conditional distribution is the same. Therefore, $p_\ell(z) = p_\ell(z')$. By plugging this into \eqref{eq:k1coarsest}, we can also show that $p_{f}(z) = p_f(z')$. Consequently, $\{p_f,p_\ell\}$ fits the definition of \eqref{eq:defncoarsest} and therefore it must be the coarsest balancing score.
		
		\item If $X_{ig} = (D_{ig},\bar{D}_{-ig})$, then $p = \{p_d,p_\ell,p_f\}$ is the coarsest score.
		
		Suppose that $p^*$ is an arbitrary balancing score. For distinct pairs $\{z,z'\}$ such that $p^*(z) = p^*(z')$ then $F(x \mid z) = F(x \mid z')$. This implies two weaker conditions $F(d \mid z) = F(D \mid z')$ and $F(\bar{D} \mid z) = F(\bar{D} \mid z')$, by projecting out the respective coordinates. Consequently $p_d(w,a) = p_d(w',a')$ and $(p_f(w,a),p_\ell(w,a)) = (p_f(w',a'),p_\ell(w',a'))$ using the results in (i) and (ii). Therefore $p(\cdot)$ fits the definition of the coarsest balancing score in \eqref{eq:defncoarsest}. This completes the proof.

	\end{enumerate}	
	
\end{proof}
